# Supplementary material for: HyGE-Occ: Hybrid View-Transformation with 3D Gaussian and Edge Priors for 3D Panoptic Occupancy Prediction
Source: arXiv:2512.19871 source file (2025-12-22)

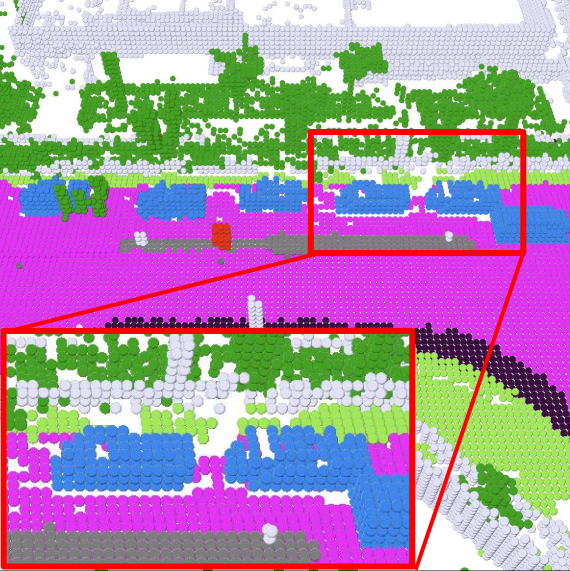

**GT**

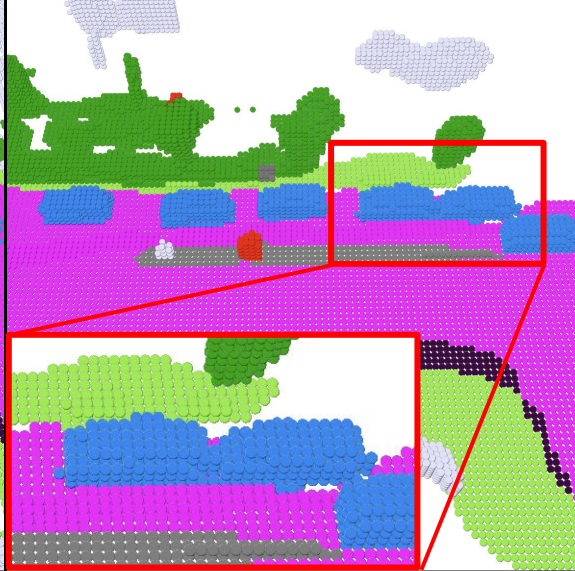

**ALOcc**

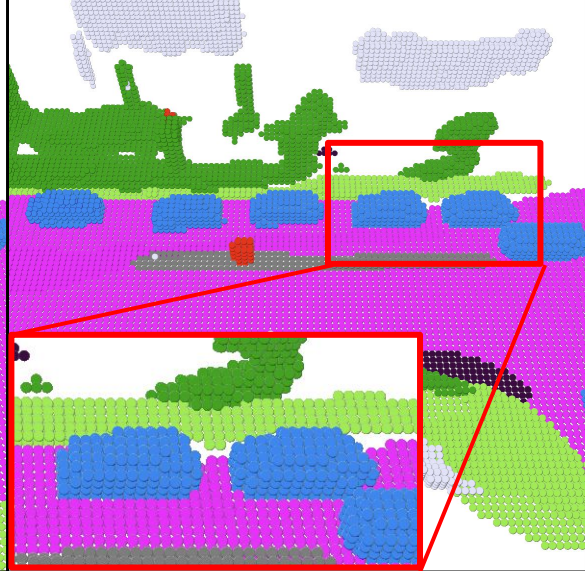

**ALOcc + HyGE-Occ**

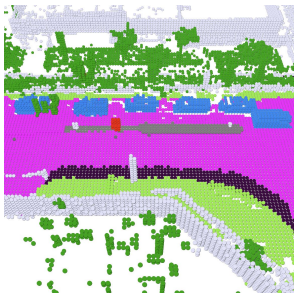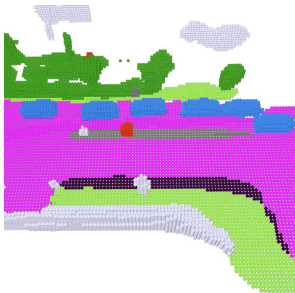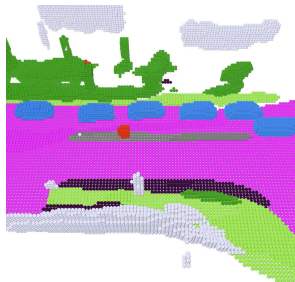

Supplement: Supplementary file 2 [file supp_Qualitative_fig_alocc.pdf]
